# Supplementary material for: PhysReaction: Physically Plausible Real-Time Humanoid Reaction Synthesis via Forward Dynamics Guided 4D Imitation
Source: arXiv:2404.01081 source file (2024-04-01)
Supplement: Supplementary file 1 [file supp.tex]

\setcounter{section}{0}
